# Supplementary material for: Unsupervised Domain Adaptation Using Feature Disentanglement And GCNs For Medical Image Classification
Source: arXiv:2206.13123 source file (2022-06-27)
Supplement: Supplementary file 1 [file Appendix.tex]

\appendix

\section{T-SNE Visualizations}
\label{app:tsne}

In Figure~\ref{fig:tsne} we show the T-sne plots for our Proposed method, for GCN2 \cite{Rev175}, DANN \cite{DANN} and our method without $L_{Str}$. The features are obtained from the final layer, and for all methods the output feature vector is $512$ dimensional, and the corresponding parameter values are $\lambda_1=0.95,\lambda_2=1.1$. The plots show visualizations for $5$ disease labels for the CheXpert dataset. We show data from the source (marked with dots) and target domain (marked with '+') for these labels. For our proposed method (Figure~\ref{fig:tsne} (a)), the source and target domain data of the same label  map to nearby areas, which indicates that the domain adaptation step successfully generates domain invariant features. Additionally, the clusters for different labels is fairly well separated. These two characteristics are not observed for the other methods. GCN2 has some level of separability but there is undesirable overlap across different different classes. The overlap across classes is even worse when we exclude the feature disentanglement components.

\rev{
The t-sne visualizations  clearly indicates that our proposed approach using feature disentanglement is highly effective in learning domain invariant representations for different disease labels. It also highlights the importance of feature disentanglement step. By separating the images into structure and texture features we are able to learn representations that have better discriminative power. 
}

\begin{figure*}[t]
 \centering
\begin{tabular}{cc}
\includegraphics[height=7.5cm, width=7.9cm]{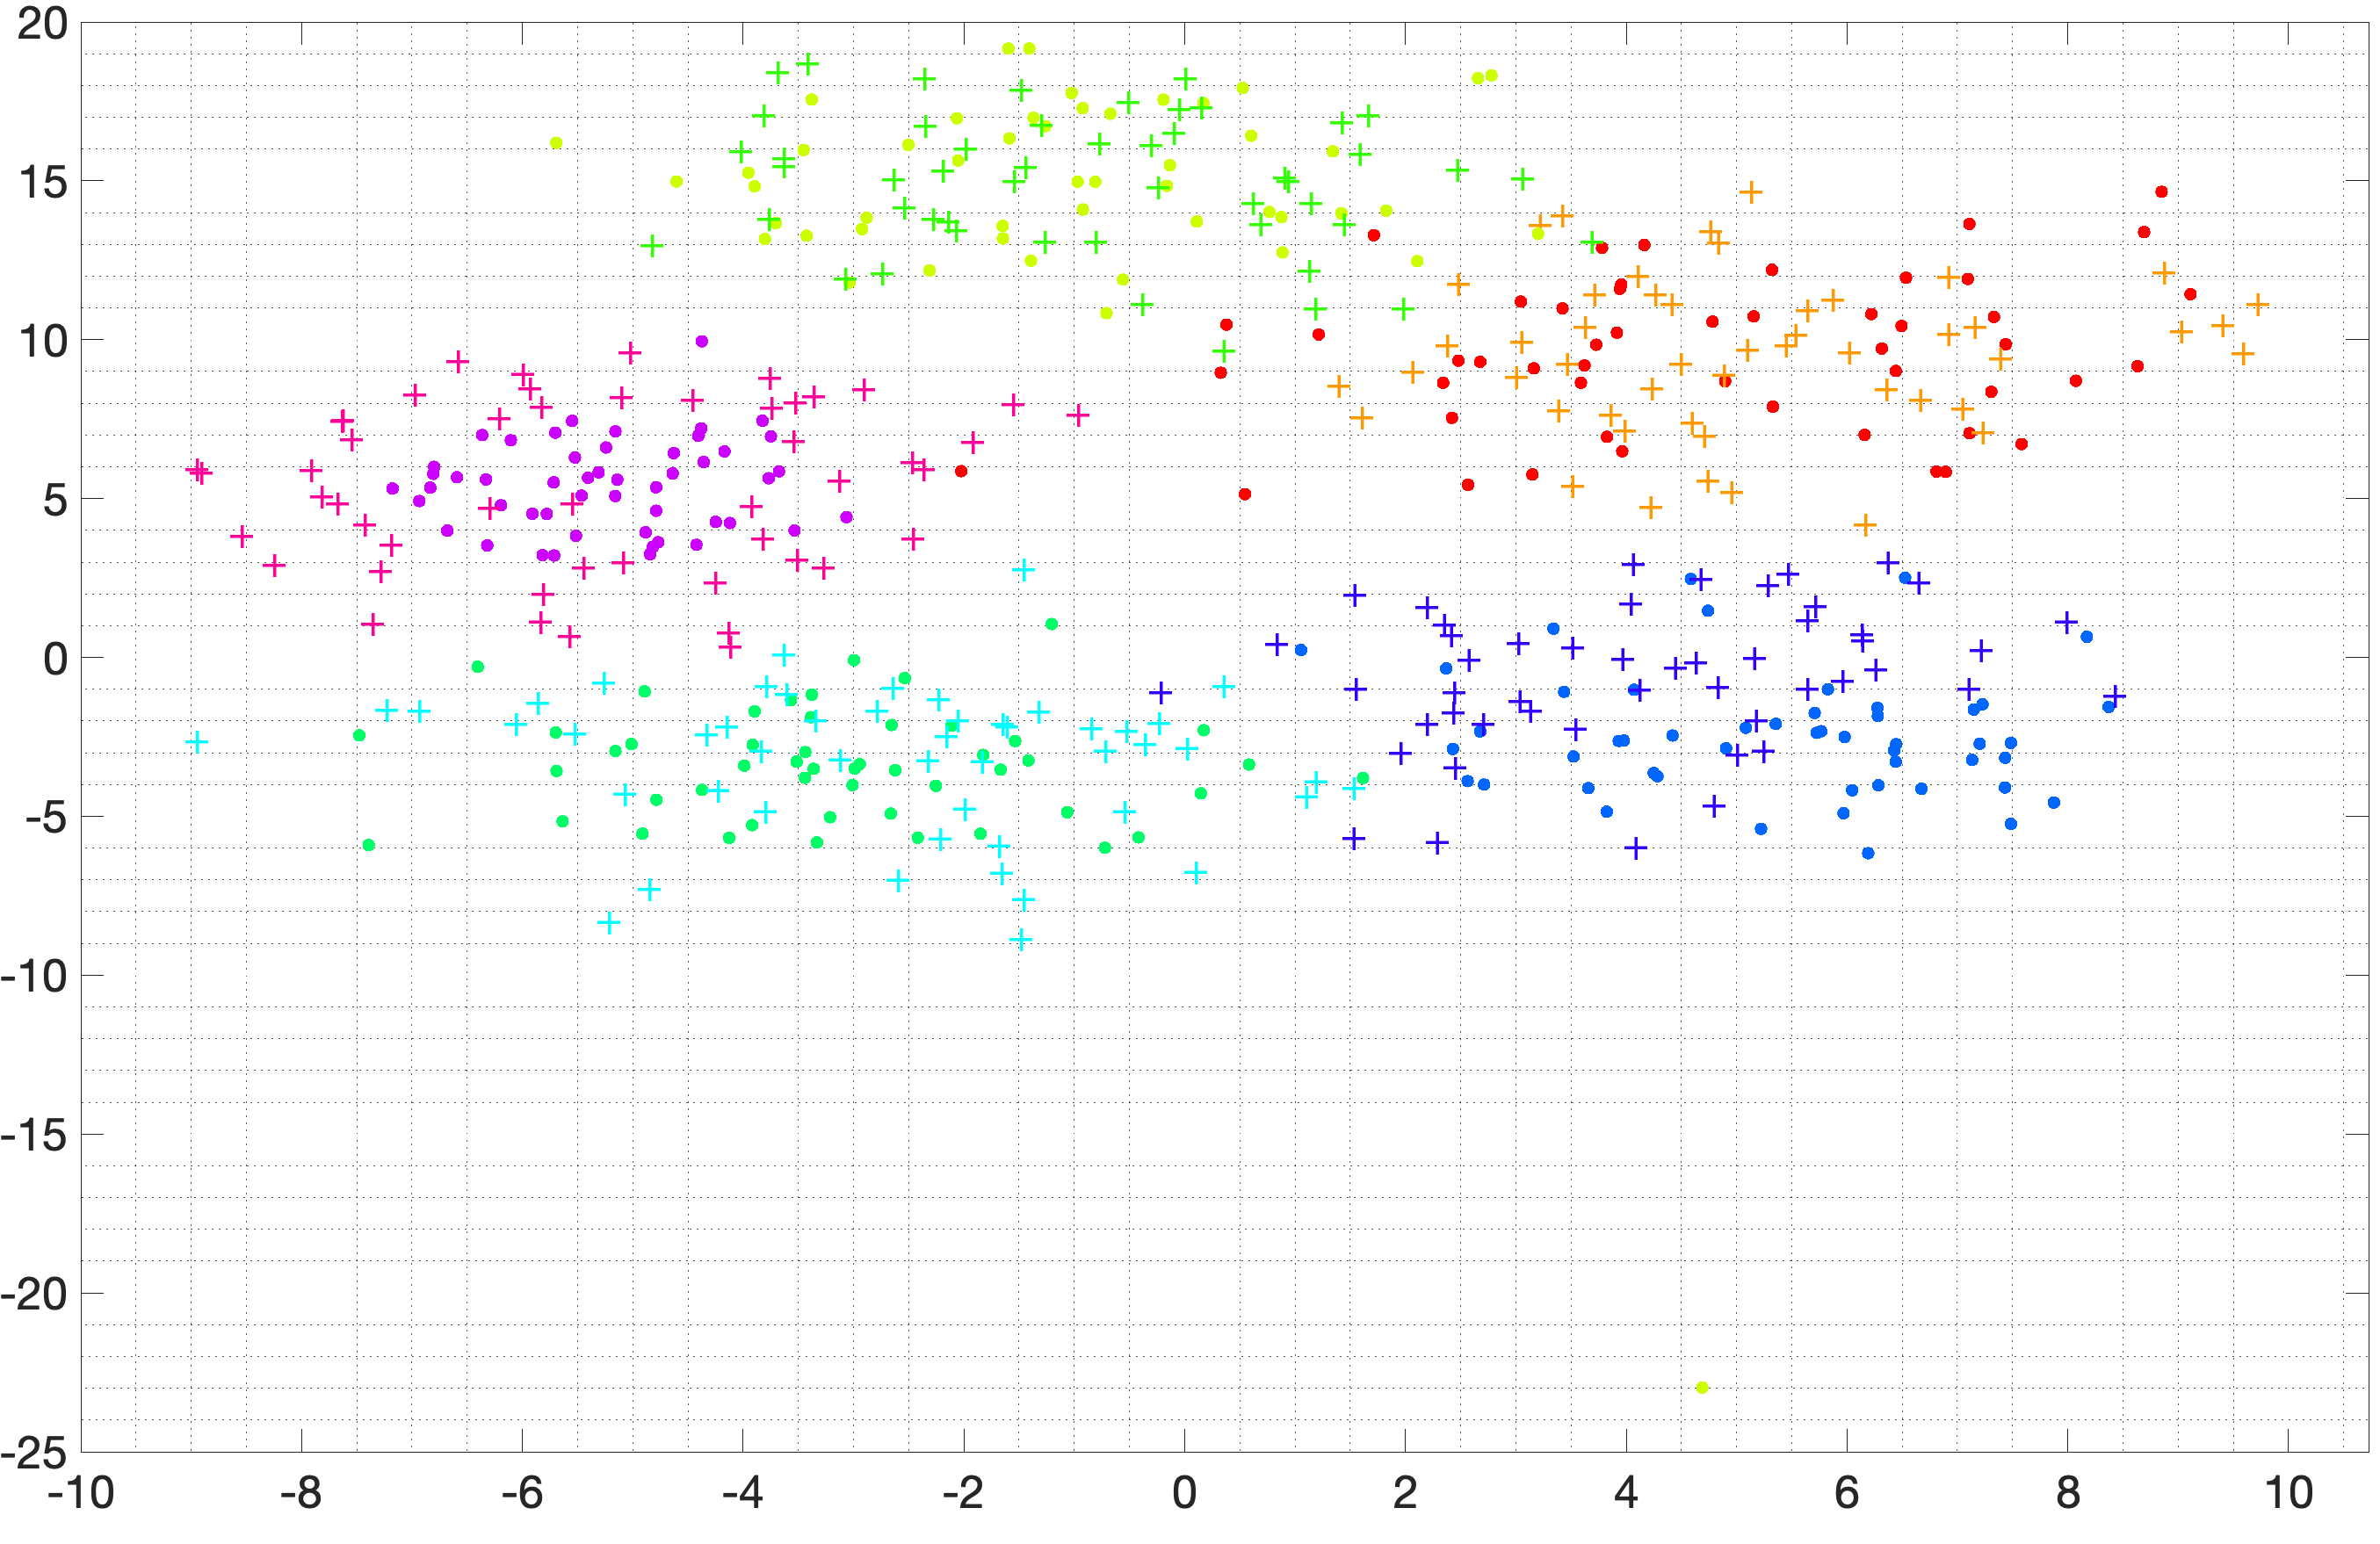} &
\includegraphics[height=7.5cm, width=7.9cm]{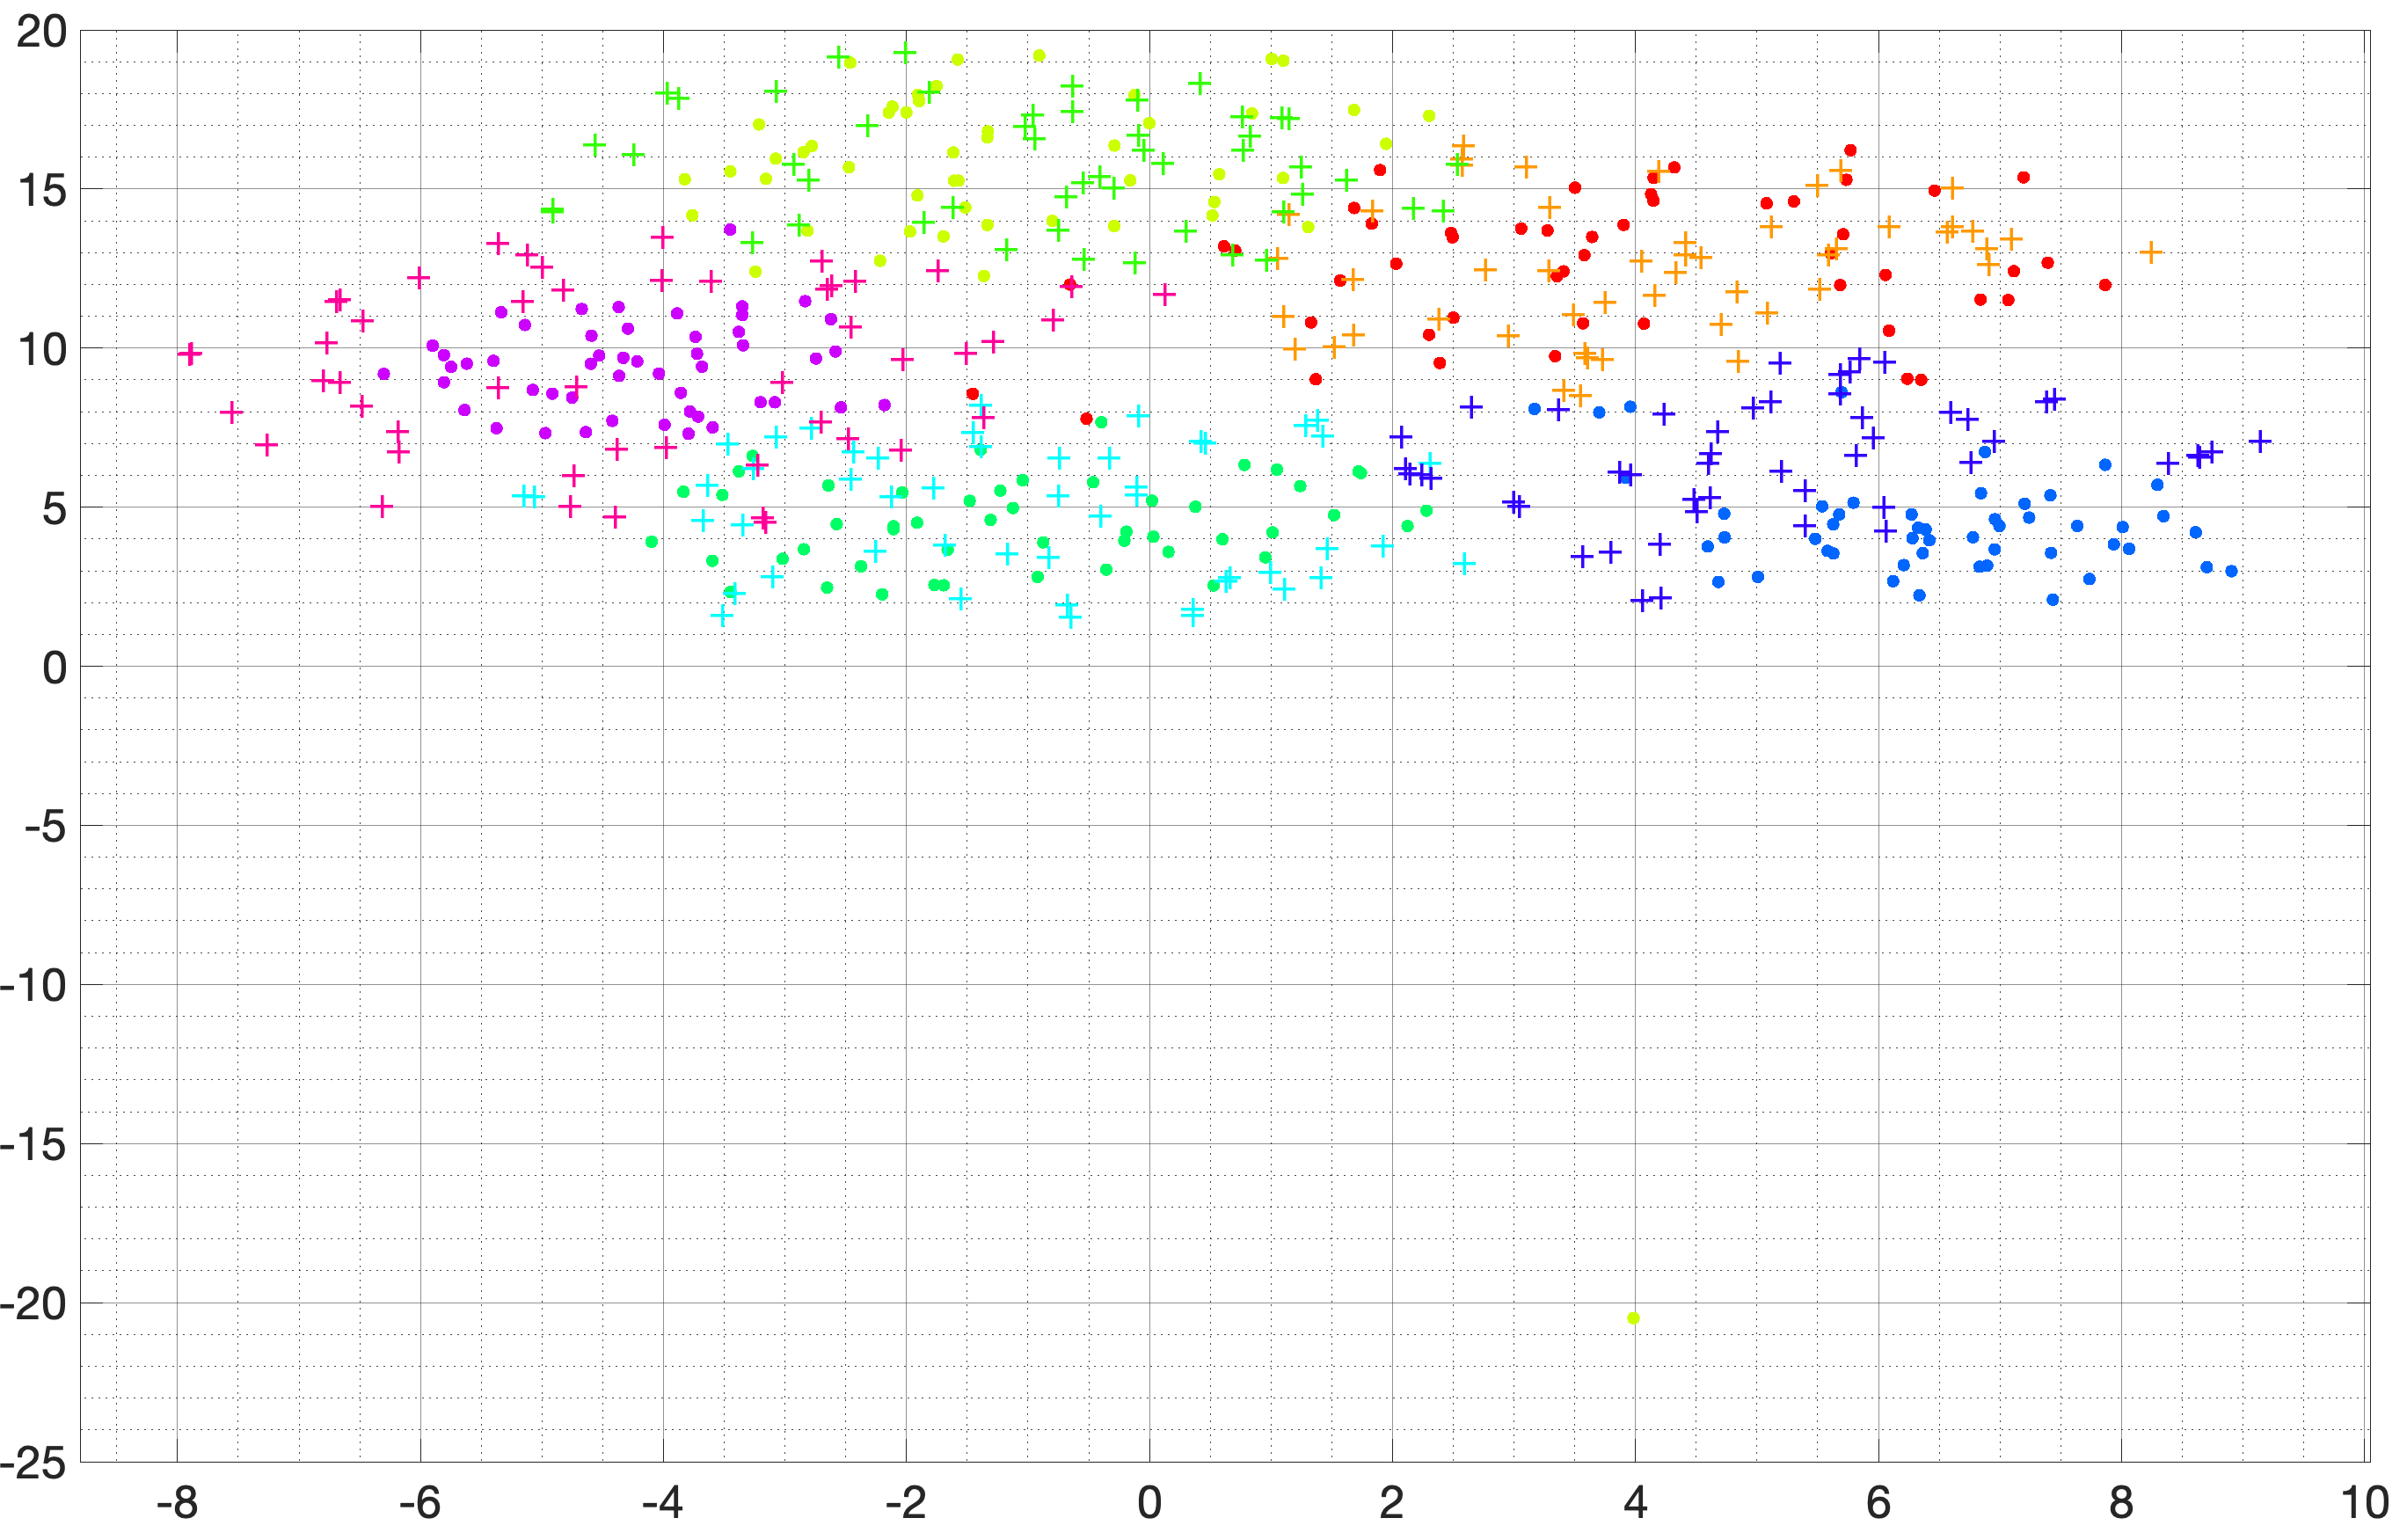} \\
(a) & (b) \\
\includegraphics[height=7.5cm, width=7.9cm]{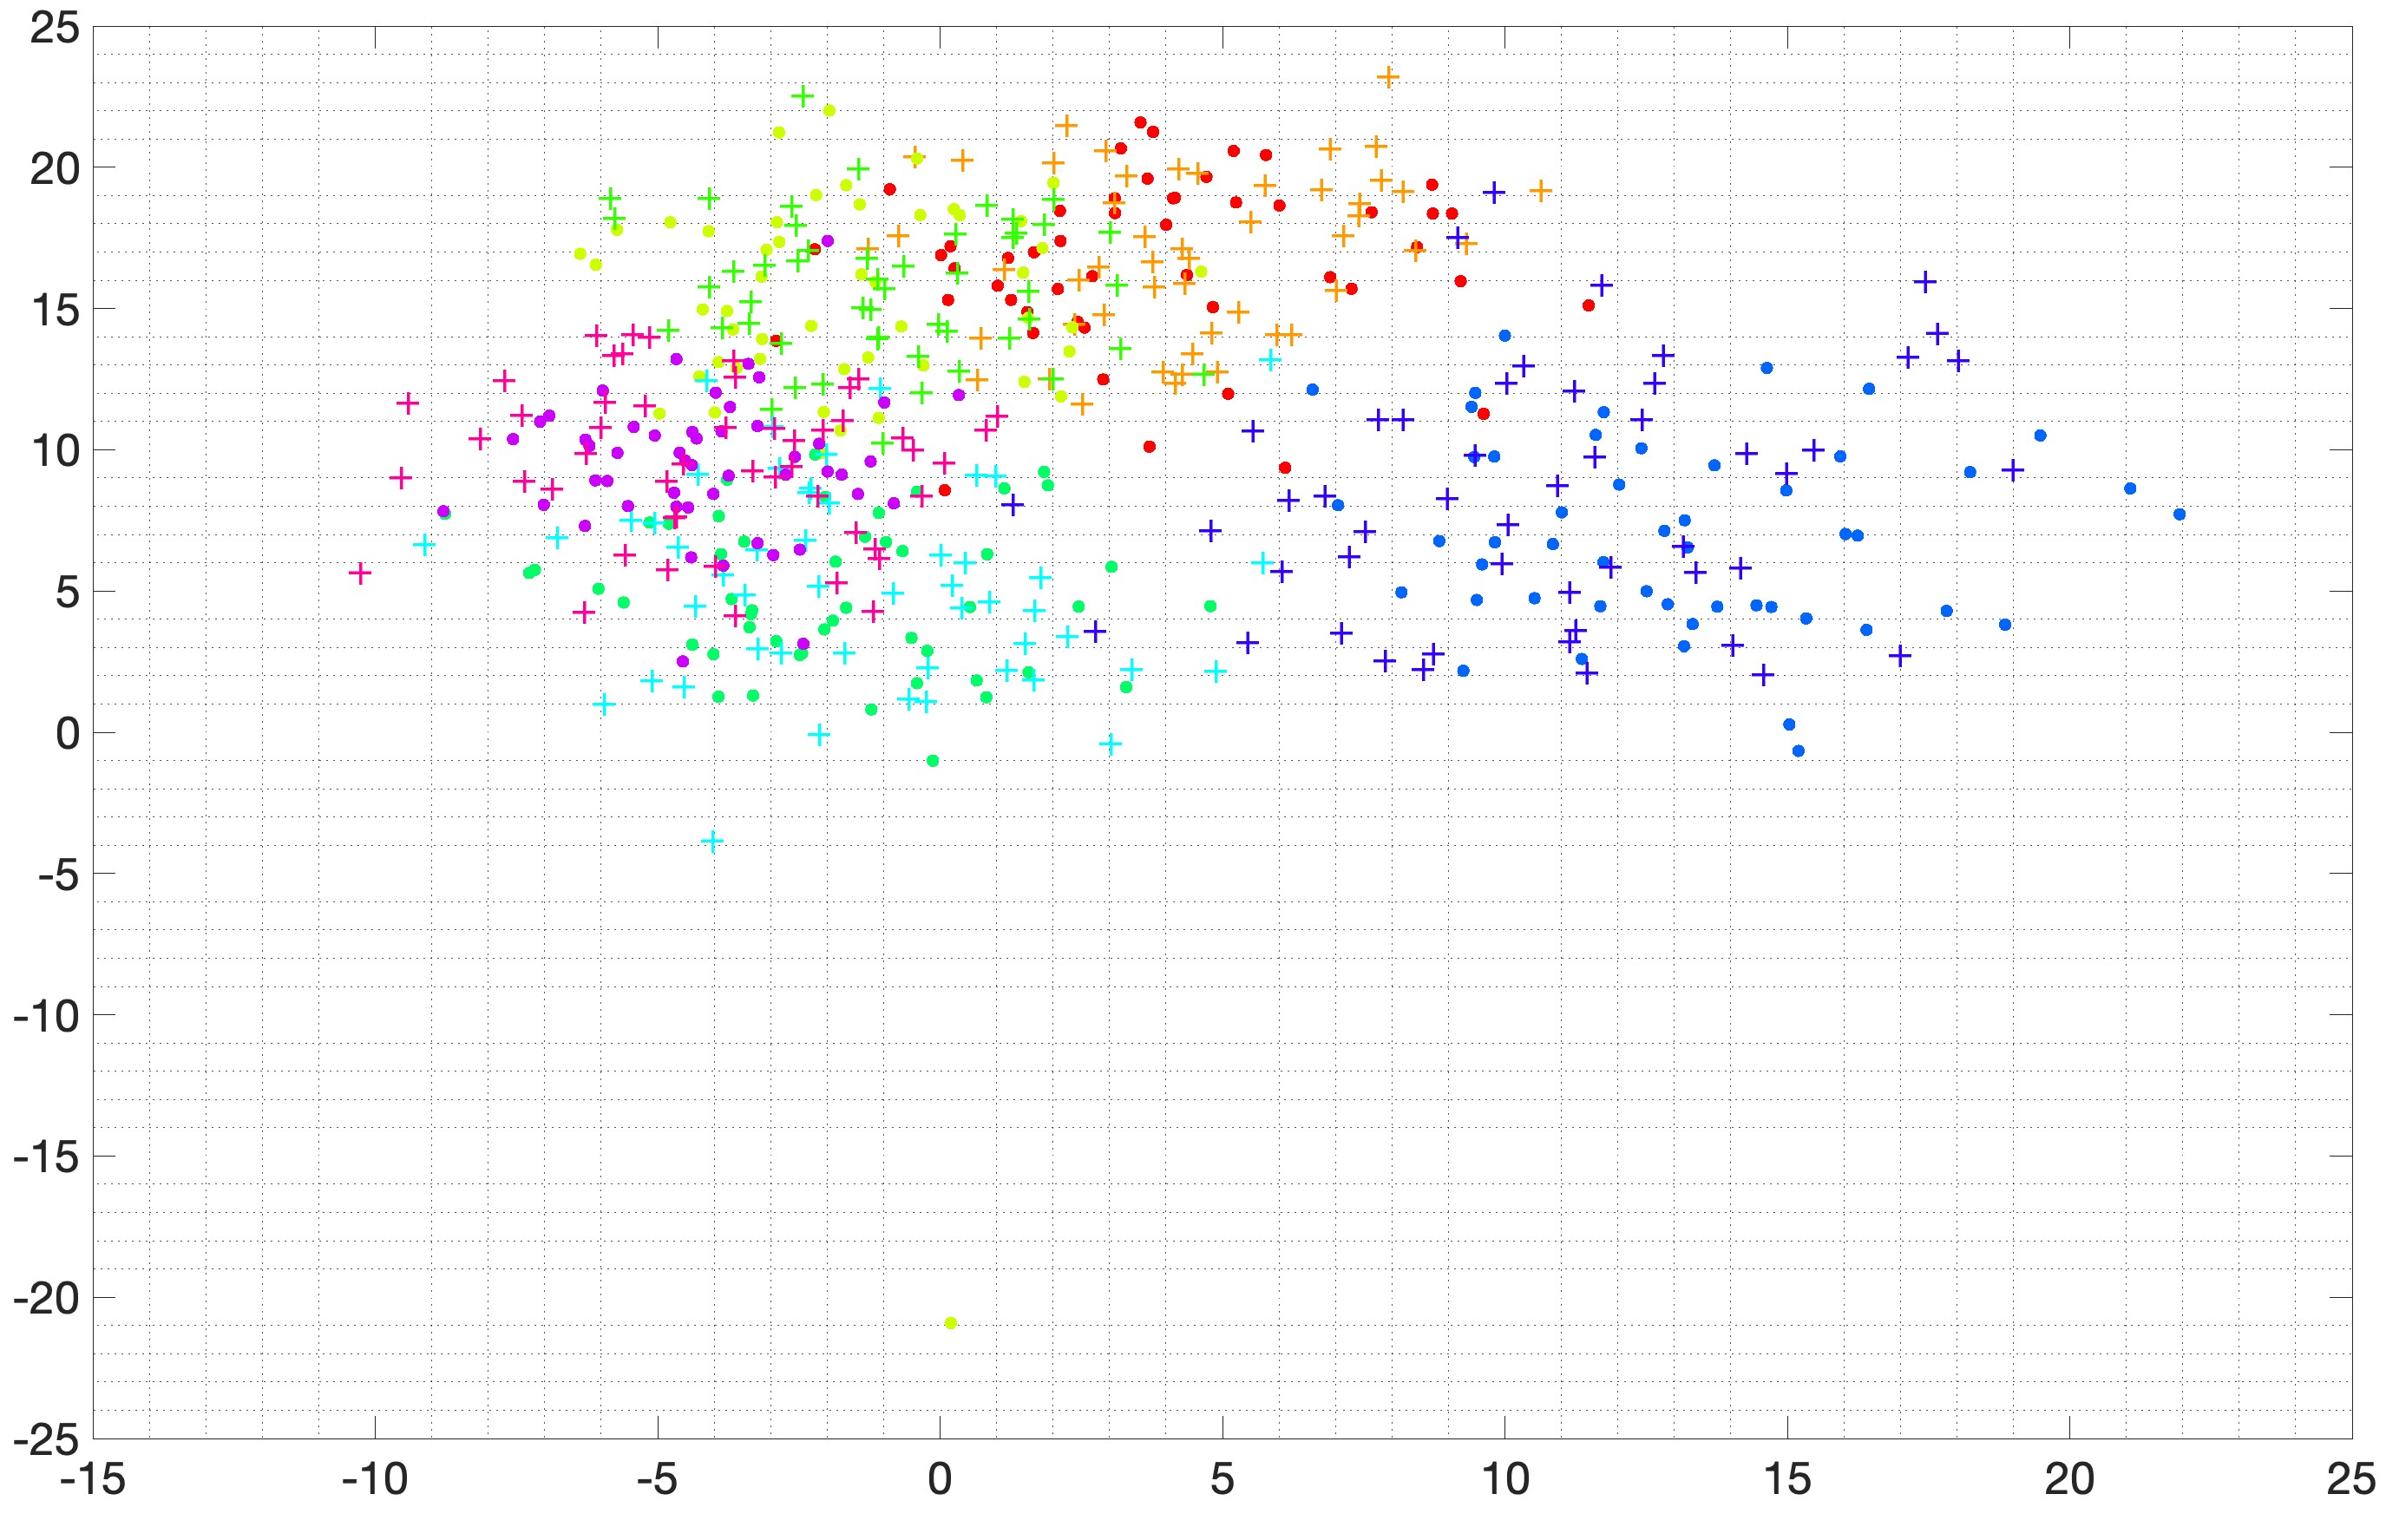} &
\includegraphics[height=7.5cm, width=7.9cm]{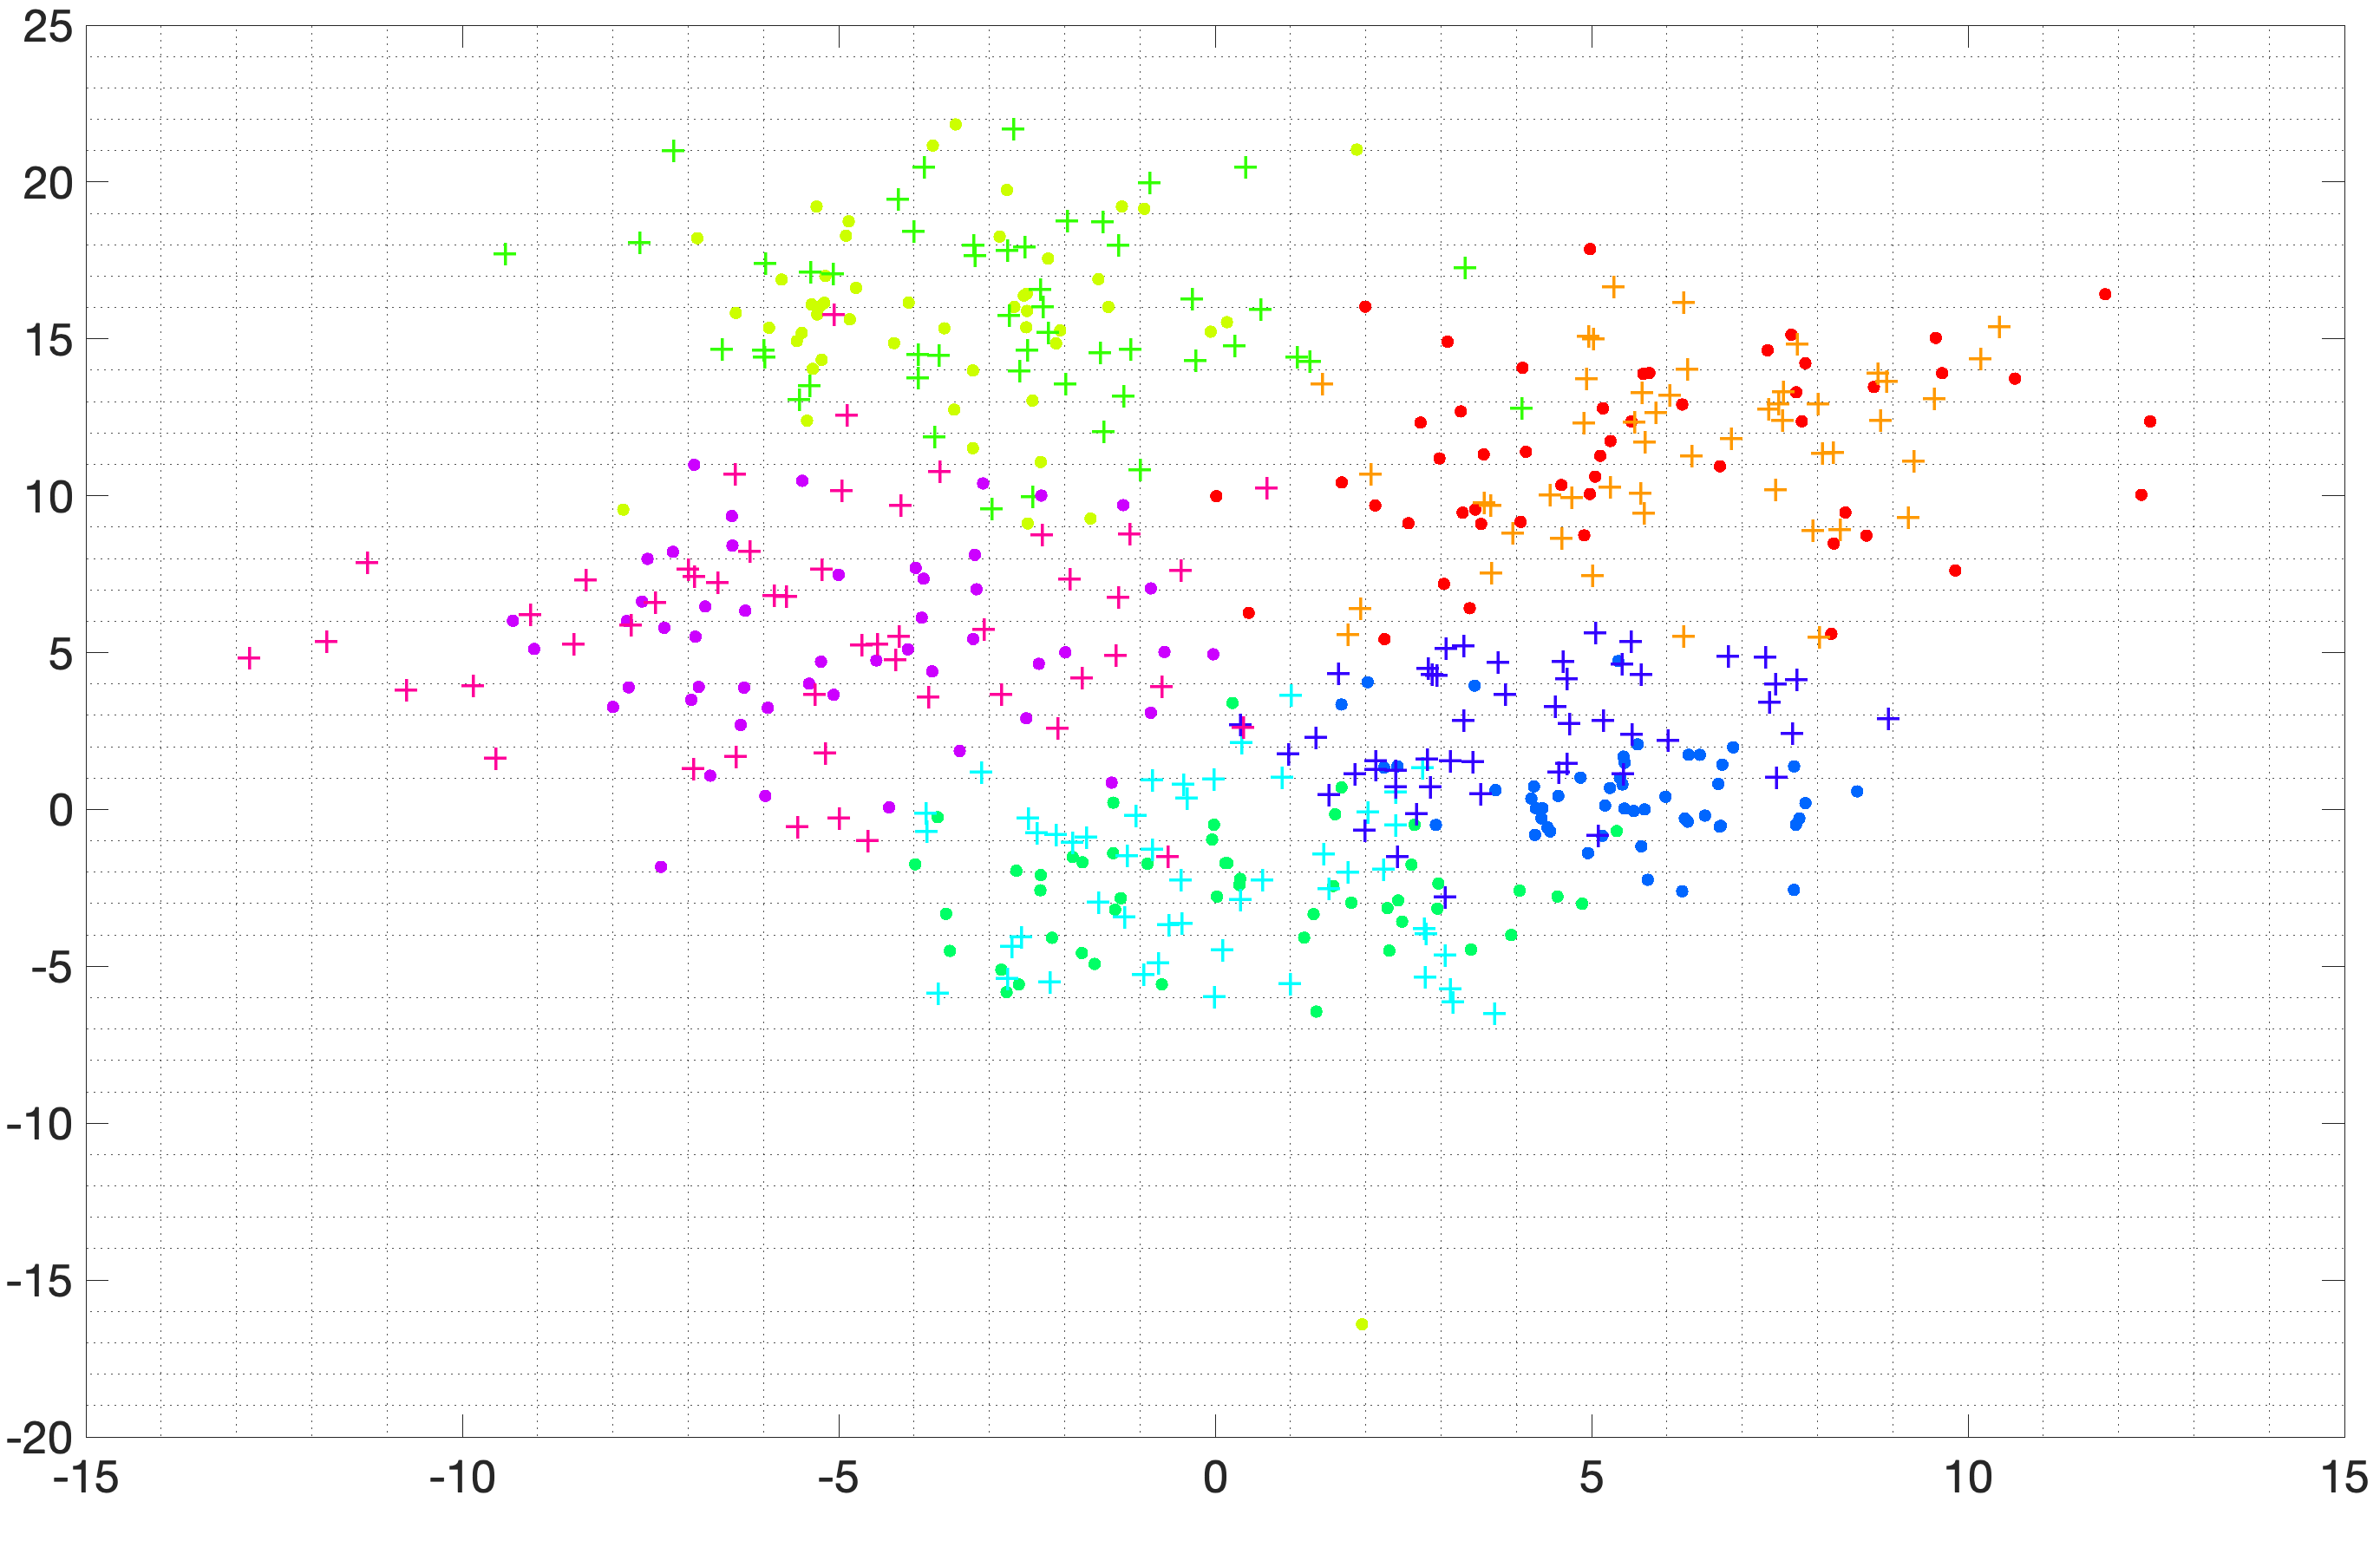} \\
 (c) & (d) \\
\end{tabular}
\begin{tabular}{c}
\includegraphics[height=1.3cm, width=15cm]{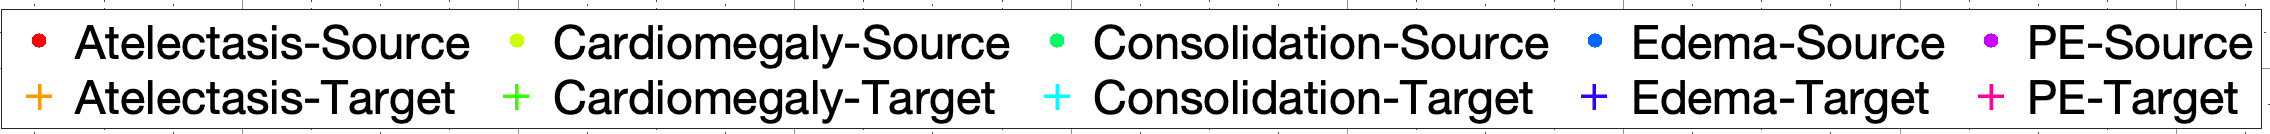}  \\
\end{tabular}
\caption{Visualization of tsne plots for different methods using 5 disease labelsfrom  the CheXpert Dataset: (a) Our proposed method; (b) Our method without using structure loss; (c) using DANN; (d) the GCN2 method of \cite{Rev175}.}
\label{fig:tsne}
\end{figure*}
